# Supplementary material for: CAN-D: A Modular Four-Step Pipeline for Comprehensively Decoding Controller Area Network Data
Source: arXiv:2006.05993 source file (2021-06-23)
Supplement: Supplementary file 1 [file appendix.tex]

\appendix

\label{sec:appendix}

\begin{figure}[ht]
    \centering
    \includegraphics[scale = .35]{figs/rpi_diagram.png}
    \caption{Simplified diagram of prototype device.}
    \label{fig:rpi_scheme}
\end{figure}
